# Supplementary material for: Faster Approximation Schemes and Parameterized Algorithms on H-Minor-Free and Odd-Minor-Free Graphs
Source: arXiv:1004.3392 source file (2010-04-20)
Supplement: Supplementary file 1 [file appendix.tex]

%-------------------------------
% Appendix
%-------------------------------

\newpage\appendix

\section{Appendix}
